# Supplementary material for: Differentiable Topology Estimating from Curvatures for 3D Shapes
Source: arXiv:2412.00140 source file (2024-11-28)
Supplement: Supplementary file 1 [file Y_suppl.tex]

\clearpage
\setcounter{page}{1}
\maketitlesupplementary

\section{Appendix}\label{appendix}

\begin{table*}[h]
\centering
\begin{tabularx}{\textwidth}{|>{\raggedright\arraybackslash}p{2cm}|X|X|X|X|X|X||X|X|X|X|X|}
\hline
Name (watertight)& Num Faces & \tabularxmulticolumncentered{5}{X||}{\vspace{0pt} \large Chamfer Distance(std)} & \tabularxmulticolumncentered{5}{X|}{\vspace{0pt}  \large Time(s)} \\ \cline{3-12} 
 &  & Diff  & 'Scan'  & Trimesh  & 'Sample'  & DOGN  &  Diff &  'Scan' &  Trimesh& 'Sample' &  DOGN \\
\hline
Rocker-arm($\checkmark$) & 20088 & \textbf{0.06632} (0.00014) & 0.08379 (0.00013) & 0.06656 (0.00013) & 0.06641 (0.00008) & 0.15448 (0.00035) & 0.4251 & 12.3401 & 10.3270 & 72.9459 & 0.3631 \\
Beast & 64618 & \textbf{0.07167} (0.00011) & 0.10516 (0.00032) & 0.07189 (0.00019) & 0.07183 (0.00034) & 0.15194 (0.00068) & 0.0075 & 14.3608 & 18.5567 & 72.6238 & 0.4087 \\
Max Planck & 99991 & \textbf{0.06057} (0.00013) & 0.35081 (0.00080) & 0.06569 (0.00022) & 0.06266 (0.00009) & 0.11371 (0.00066) & 0.0065 & 16.9182 & 102.0209 & 76.7355 & 0.5564 \\
Lucy($\checkmark$) & 99970 & 0.05977 (0.00016) & 0.07760 (0.00038) & \textbf{0.05945} (0.00004) & 0.05951 (0.00026) & 0.15320 (0.00027) & 0.0062 & 16.3613 & 66.0559 & 71.7929 & 0.4569 \\
Cheburashka($\checkmark$) & 13334 & \textbf{0.06254} (0.00012) & 0.08655 (0.00028) & 0.06275 (0.00019) & 0.06270 (0.00024) & 0.16430 (0.00055) & 0.0045 & 12.6865 & 3.1635 & 72.2148 & 0.3245 \\
Happy & 98601 & 0.05548 (0.00013) & 0.08143 (0.00032) & 0.05548 (0.00021) & \textbf{0.05537} (0.00007) & 0.16028 (0.00066) & 0.0073 & 17.0295 & 23.5146 & 71.7547 & 0.4803 \\

Teapot & 6320 & \textbf{0.05685} (0.00006) & 0.12914 (0.00071) & 0.05716 (0.00021) & 0.06477 (0.00012) & 0.16999 (0.00031) & 0.0046 & 11.7145 & 4.4557 & 72.3538 & 0.3307 \\

Bimba($\checkmark$) & 224906 & 0.05728 (0.00014) & 0.10217 (0.00025) & \textbf{0.05718} (0.00021) & \textbf{0.05718} (0.00013) & 0.16595 (0.00026) & 0.3337 & 20.9800 & 244.5197 & 75.5195 & 0.7512 \\

Igea($\checkmark$) & 268686 & 0.06211 (0.00006) & 0.13745 (0.00031) & \textbf{0.06203} (0.00016) & 0.06215 (0.00003) & 0.18204 (0.00030) & 3.6248 & 24.0900 & 469.7210 & 78.1245 & 0.8369 \\

Hourse($\checkmark$) & 96966 & \textbf{0.06970 (0.00013)} & 0.12735 (0.00030) & 0.07019 (0.00007) & 0.10821 (0.00067) & 0.15961 (0.00018) & 0.0072 & 16.3146 & 87.9119 & 74.2368 & 0.4593 \\

Homer($\checkmark$) & 12000 & 0.05890 (0.00005) & 0.07347 (0.00025) & 0.05876 (0.00017) & \textbf{0.05841} (0.00020) & 0.15538 (0.00039) & 0.0063 & 11.2691 & 2.3533 & 74.2110 & 0.3246 \\

Spot & 5856 & \textbf{0.06440} (0.00007) & 0.10161 (0.00046) & 0.06463 (0.00017) & 0.06449 (0.00016) & 0.16768 (0.00032) & 0.0062 & 11.5103 & 9.6123 & 69.0767 & 0.3217 \\

Armadillo($\checkmark$) & 99976 & 0.07081 (0.00001) & 0.11524 (0.00024) & \textbf{0.07046} (0.00028) & 0.07061 (0.00021) & 0.16688 (0.00056) & 0.0055 & 16.8934 & 121.1818 & 71.5409 & 0.5164 \\

Suzanne & 968 & 0.06440 (0.00024) & 0.10288 (0.00031) & 0.06312 (0.00003) & \textbf{0.06173} (0.00017) & 0.17534 (0.00040) & 0.0064 & 12.1686 & 1.2807 & 69.1196 & 0.3132 \\
Stanford Bunny & 69451 & \textbf{0.06344} (0.00011) & 0.15924 (0.00045) & 0.06814 (0.00024) & 0.06364 (0.00020) & 0.12063 (0.00026) & 0.0074 & 16.2307 & 81.7012 & 71.1485 & 0.5156 \\
Nefertiti($\checkmark$) & 99938 & 0.05991 (0.00011) & 0.08721 (0.00039) & \textbf{0.05972} (0.00022) & 0.06000 (0.00023) & 0.16238 (0.00036) & 0.0055 & 17.6811 & 104.9907 & 75.9086 & 0.4892 \\
Ogre & 124008 & 0.06791 (0.00030) & 0.09158 (0.00013) & \textbf{0.06654} (0.00024) & 0.06862 (0.00033) & 0.15788 (0.00040) & 0.0086 & 18.0386 & 12.8931 & 72.2672 & 0.5144 \\
Cow($\checkmark$) & 5804 & \textbf{0.06242} (0.00011) & 0.21833 (0.00130) & 0.06272 (0.00007) & 0.17479 (0.00264) & 0.15892 (0.00036) & 0.0048 & 12.1376 & 1.2943 & 69.5902 & 0.2743 \\
Fandisk($\checkmark$) & 12946 & \textbf{0.05456} (0.00016) & 0.09516 (0.00026) & 0.05460 (0.00005) & 0.05467 (0.00001) & 0.16631 (0.00063) & 0.0047 & 13.4979 & 6.9413 & 69.3316 & 0.3324 \\
Car& 157384& 0.07015 (0.00014)&  0.08850 (0.00011) &  \textbf{0.06765} (0.00013) & 0.07037 (0.00034)&0.23775 (0.00040)& 3.8466 & 20.1299 &799.0143 & 76.3597 & 0.7136 \\
Tableware&  4788& 0.63220 (0.00228) & 0.21702 (0.00033) &  0.62292 (0.00127)& 0.62329 (0.00116) & \textbf{0.17387} (0.00065) &0.0062 &11.5668 & 3.6265& 72.8735& 0.3134\\
Ladder & 828 & 0.28433 (0.00046) & 0.29627 (0.00090)  &0.28649 (0.00112) & 0.28678 (0.00136) & \textbf{0.13036} (0.00032) & 0.1531 &12.5374 & 0.08043 & 70.7119 & 0.2595\\
Bull & 2418 & 0.06685 (0.00029) & 0.21340 (0.00072) & \textbf{0.06670} (0.00023) & 0.13797 (0.00081)&0.16155 (0.00028) &  0.0047& 11.6457& 2.0163&74.1523 &0.3395\\
\hline
\end{tabularx}
\caption{Resulting Chamfer Distances and Computation Times of Different Methods for resolution 32}
\label{resol32}
\end{table*}

\begin{table*}[!h]
\centering
\begin{tabularx}{\textwidth}{|>{\raggedright\arraybackslash}p{2cm}|X|X|X|X|X|X||X|X|X|X|X|}
\hline
Name (watertight) & Num Faces & \tabularxmulticolumncentered{5}{X||}{\vspace{0pt} \large Chamfer Distance(std)} & \tabularxmulticolumncentered{5}{X|}{\vspace{0pt}  \large Time(s)} \\ \cline{3-12} 
 &  & Diff  & 'Scan'  & Trimesh  & 'Sample'  & DOGN  &  Diff &  'Scan' &  Trimesh& 'Sample' &  DOGN \\
\hline
Rocker-arm($\checkmark$) & 20088 & \textbf{0.03568} (0.00009) & 0.06522 (0.00018) & 0.03569 (0.00005) & 0.03575 (0.00010) & 0.08130 (0.00028) & 3.10 & 15.80 & 97.47 & 470.83 & 1.90 \\
Beast & 64618 & 0.03357 (0.00002) & 0.07294 (0.00014) & \textbf {0.03351} (0.00006) & 0.03761 (0.00013) & 0.07956 (0.00020) & 9.04 & 18.61 & 147.10 & 479.61 & 2.04 \\
Max Planck & 99991 & \textbf{0.03495} (0.00006) & 0.35516 (0.00073) & 0.03995 (0.00022) & 0.03806 (0.00009) & 0.05998 (0.00022) & 14.30 & 22.87 & 806.17 & 500.46 & 2.56 \\
Lucy($\checkmark$) & 99970 & \textbf{0.03114} (0.00005) & 0.05217 (0.00014) & 0.03122 (0.00006) & 0.03122 (0.00011) & 0.07905 (0.00018) & 14.07 & 19.51 & 574.55 & 479.88 & 1.99 \\
Cheburashka($\checkmark$) & 13334 & 0.03594 (0.00007) & 0.07236 (0.00033) & \textbf{0.03584} (0.00005) & 0.03607 (0.00010) & 0.08458 (0.00022) & 1.46 & 16.67 & 26.07 & 474.34 & 2.16 \\
Happy & 98601 & 0.03270 (0.00014) & 0.06755 (0.00029) & \textbf{0.03266} (0.00004) & 0.03296 (0.00007) & 0.07941 (0.00042) & 13.89 & 20.64 & 188.29 & 488.89 & 2.17 \\
Teapot & 6320 & \textbf{0.03291} (0.00014) & 0.16490 (0.00093) & 0.03879 (0.00005) & 0.04875 (0.00032) & 0.08601 (0.00013) & 0.70 & 19.10 & 35.85 & 480.15 & 2.01 \\
Bimba($\checkmark$) & 224906 & \textbf{0.03427} (0.00007) & 0.09563 (0.00037) & 0.03432 (0.00007) & 0.03445 (0.00012) & 0.08473 (0.00016) & 41.03 & 27.55 & 2199.34 & 497.14 & 2.74 \\
Igea($\checkmark$) & 268686 & \textbf{0.03663} (0.00006) & 0.13448 (0.00028) & * & 0.03677 (0.00004) & 0.09399 (0.00016) & 52.59 & 31.82 & $>$4000 & 507.74 & 2.86 \\
Hourse($\checkmark$) & 96966 & \textbf{0.03598} (0.00003) & 0.09547 (0.00043) & 0.03605 (0.00011) & 0.06874 (0.00072) & 0.08316 (0.00024) & 15.53 & 22.91 & 791.05 & 484.71 & 2.14 \\
Homer($\checkmark$) & 12000 & 0.03298 (0.00012) & 0.05691 (0.00013) & \textbf{0.03292} (0.00010) & \textbf{0.03292} (0.00007) & 0.07907 (0.00023) & 1.32 & 15.76 & 16.25 & 472.65 & 1.89 \\
Spot & 5856 & 0.03628 (0.00006) & 0.09217 (0.00013) & \textbf{0.03627} (0.00009) & 0.03637 (0.00007) & 0.08544 (0.00015) & 0.65 & 19.74 & 81.19 & 478.09 & 2.05 \\
Armadillo($\checkmark$) & 99976 & 0.03737 (0.00005) & 0.08675 (0.00014) & \textbf{0.03718} (0.00003) & 0.03747 (0.00005) & 0.08546 (0.00012) & 14.07 & 22.15 & 1001.82 & 478.16 & 2.32 \\
Suzanne & 968 & \textbf{0.03614} (0.00006) & 0.09256 (0.00036) & 0.03983 (0.00010) & 0.03779 (0.00004) & 0.08982 (0.00033) & 0.11 & 17.65 & 11.48 & 474.98 & 1.87 \\
Stanford Bunny & 69451 & \textbf{0.03847} (0.00014) & 0.16958 (0.00151) & 0.04645 (0.00009) & 0.03997 (0.00008) & 0.06325 (0.00006) & 9.76 & 22.77 & 669.95 & 475.62 & 2.50 \\
Nefertiti($\checkmark$) & 99938 & 0.03345 (0.00007) & 0.07886 (0.00014) & \textbf{0.03337} (0.00005) & 0.03340 (0.00004) & 0.08305 (0.00033) & 14.07 & 24.16 & 908.54 & 503.51 & 2.30 \\
Ogre & 124008 & 0.03485 (0.00010) & 0.07289 (0.00002) & \textbf{0.03426} (0.00002) & 0.03705 (0.00017) & 0.08312 (0.00016) & 19.13 & 21.47 & 126.22 & 481.03 & 2.20 \\
Cow($\checkmark$) & 5804 & \textbf{0.03376} (0.00008) & 0.20966 (0.00108) & 0.03378 (0.00014) & 0.20101 (0.00081) & 0.07951 (0.00016) & 0.64 & 16.63 & 8.24 & 462.41 & 1.82 \\
Fandisk($\checkmark$) & 12946 & 0.04016 (0.00002) & 0.08417 (0.00022) & \textbf{0.04015} (0.00004) & 0.04017 (0.00004) & 0.07795 (0.00006) & 1.42 & 16.30 & 61.16 & 462.34 & 1.86 \\
Car & 157384&  0.04826 (0.00005)& 0.08326 (0.00029) & \textbf{0.04268} (0.00011)& 0.05191 (0.00005) & 0.14442 (0.00060) & 28.38&  23.19 & 2187.78 & 518.36 & 2.89\\
Tableware &  4788& \textbf{0.11128} (0.00041) & 0.18683 (0.00079) & 0.11143 (0.00022)& 0.11268 (0.00042)& 0.11983 (0.00033)&  0.53 &15.02 & 36.45 & 496.58&1.79\\
 Ladder &  828& 0.13856 (0.00010) & 0.23965 (0.00057)  & 0.13874 (0.00061)& 0.13813 (0.00036) &\textbf{0.07570} (0.00018)   &0.39 & 14.08 &  0.25 &482.66 &1.60\\
 Bull&  2418&0.03542 (0.00003) & 0.19739 (0.00125) &  \textbf{0.03541} (0.00003) &0.15641 (0.00064)&0.08279 (0.00019) &0.27 & 16.94 & 18.02& 521.10& 2.13\\
\hline
\end{tabularx}
\caption{Resulting Chamfer Distances and Computation Times of Different Methods for resolution 64}
\label{resol64}
\end{table*}

\begin{table*}[!h]
\centering
\begin{tabularx}{\textwidth}{|>{\raggedright\arraybackslash}p{2cm}|X|X|X|X|X||X|X|X|X|X|X|}
\hline
Name (watertight) & \tabularxmulticolumncentered{5}{X||}{\vspace{0pt} \large Hausdorff Distance (resol 32)} & \tabularxmulticolumncentered{5}{X|}{\vspace{0pt} \large Hausdorff Distance (resol 64)} \\ \cline{1-11} 
 & Diff  & 'Scan'  & 'Sample'  & 'Trimesh'  & DOGN & Diff  & 'Scan'  & 'Sample'  & 'Trimesh'  & DOGN \\
\hline
Rocker-arm&0.09804 (0.00028)&0.13694 (0.00051)&0.09833 (0.00058)&\textbf{0.09783} (0.00067)&0.21022 (0.00181)&0.04585 (0.00121)&0.11573 (0.00410)&\textbf{0.04443} (0.00119)&0.04651 (0.00053)&0.11563 (0.00050)\\
Beast&0.19894 (0.00107)&0.26045 (0.00093)&\textbf{0.19595} (0.00437)&0.20010 (0.00071)&0.23835 (0.00123)&0.08119 (0.00133)&0.13537 (0.00088)&\textbf{0.07804} (0.00296)&0.45707 (0.00260)&0.11417 (0.00135)\\
Max Planck&\textbf{0.17962} (0.00315)&1.09022 (0.00811)&0.27223 (0.00228)&0.22204 (0.00199)&0.21338 (0.00105)&0.17761 (0.00241)&1.07249 (0.00551)&0.26696 (0.00174)&0.63863 (0.00107)&\textbf{0.10693} (0.00124)\\
Lucy&\textbf{0.15998} (0.00132)&0.16109 (0.00193)&0.16288 (0.00137)&0.16278 (0.00154)&0.21806 (0.00112)&\textbf{0.06911} (0.00104)&0.12530 (0.00233)&0.07138 (0.00029)&0.07018 (0.00013)&0.12193 (0.00040)\\
Cheburashka&0.11699 (0.00068)&0.15871 (0.00131)&\textbf{0.11667} (0.00124)&0.11675 (0.00073)&0.22699 (0.00259)&\textbf{0.08833} (0.00058)&0.13572 (0.00356)&0.08870 (0.00190)&0.17981 (0.00110)&0.14794 (0.00174)\\
Happy&0.12999 (0.00068)&0.14404 (0.00079)&0.12847 (0.00076)&\textbf{0.12702} (0.00251)&0.23513 (0.00134)&\textbf{0.06669} (0.00260)&0.12116 (0.00037)&0.07515 (0.00332)&0.13735 (0.00163)&0.11438 (0.00161)\\
Teapot&\textbf{0.11404} (0.00119)&1.03774 (0.00159)&0.29660 (0.00184)&0.29425 (0.00041)&0.27024 (0.00118)&\textbf{0.11140} (0.00194)&1.03101 (0.01343)&0.25777 (0.00379)&0.35074 (0.00100)&0.15234 (0.00113)\\
Bimba&0.10842 (0.00251)&0.17430 (0.00183)&\textbf{0.10810} (0.00163)&0.13392 (0.00679)&0.27758 (0.00387)&0.05352 (0.00076)&0.14291 (0.00019)&\textbf{0.05123} (0.00114)&0.12672 (0.05122)&0.13154 (0.00089)\\
Igea&\textbf{0.08470} (0.00083)&0.16438 (0.00067)&0.08807 (0.00486)&0.08518 (0.00137)&0.22979 (0.00164)&0.04855 (0.00181)&0.12874 (0.00058)&*&\textbf{0.04498} (0.00081)&0.11116 (0.00069)\\
Horse&0.12941 (0.00116)&0.66342 (0.00346)&\textbf{0.12695} (0.00019)&0.69284 (0.00014)&0.22085 (0.00111)&0.05391 (0.00248)&0.62432 (0.00143)&\textbf{0.05171} (0.00058)&0.70203 (0.00186)&0.10906 (0.00110)\\
Homer&0.09541 (0.00109)&0.14960 (0.00024)&0.09477 (0.00110)&\textbf{0.09332} (0.00086)&0.20811 (0.00181)&0.05552 (0.00177)&0.12214 (0.00030)&\textbf{0.05250} (0.00038)&0.05271 (0.00154)&0.13304 (0.00102)\\
Spot&\textbf{0.09370} (0.00125)&0.14076 (0.00066)&0.09496 (0.00147)&0.09580 (0.00093)&0.21575 (0.00071)&0.04495 (0.00060)&0.12255 (0.00149)&\textbf{0.04177} (0.00042)&0.04207 (0.00109)&0.10402 (0.00070)\\
Armadillo&0.16884 (0.00294)&0.18805 (0.00160)&\textbf{0.16510} (0.00644)&0.16510 (0.00147)&0.22296 (0.00237)&0.07307 (0.00485)&0.13891 (0.00158)&\textbf{0.06400} (0.00390)&0.54865 (0.00217)&0.10959 (0.00144)\\
Suzanne&\textbf{0.12759} (0.00192)&0.59997 (0.00491)&0.19467 (0.00321)&0.37024 (0.00129)&0.27440 (0.00019)&\textbf{0.09585} (0.00327)&0.58307 (0.00278)&0.23128 (0.00116)&0.48175 (0.00127)&0.15865 (0.00179)\\
Stanford Bunny&\textbf{0.10395} (0.00281)&0.70338 (0.00362)&0.21473 (0.00037)&0.23383 (0.00432)&0.20713 (0.00074)&\textbf{0.09856} (0.00482)&0.84165 (0.01241)&0.23335 (0.00226)&0.36202 (0.00408)&0.10329 (0.00120)\\
Nefertiti&\textbf{0.09277} (0.00073)&0.14624 (0.00248)&0.09496 (0.00052)&0.09448 (0.00147)&0.21426 (0.00053)&\textbf{0.05853} (0.00330)&0.11916 (0.00113)&0.06024 (0.00078)&0.27661 (0.12798)&0.10759 (0.00192)\\
Ogre&0.15168 (0.00076)&0.16781 (0.00221)&\textbf{0.15102} (0.00196)&0.15623 (0.00155)&0.21357 (0.00012)&0.09467 (0.00219)&0.12800 (0.00029)&\textbf{0.06594} (0.00024)&0.16643 (0.00068)&0.15010 (0.00145)\\
Cow&0.17486 (0.00357)&1.02813 (0.00055)&\textbf{0.17444} (0.00070)&1.05163 (0.00121)&0.21426 (0.00136)&\textbf{0.08899} (0.00295)&0.96566 (0.00043)&0.09079 (0.00102)&0.99838 (0.00161)&0.10803 (0.00122)\\
Fandisk&0.10267 (0.00184)&0.12448 (0.00245)&\textbf{0.09604} (0.00439)&0.10156 (0.00174)&0.20640 (0.00104)&0.06248 (0.00573)&0.22357 (0.00603)&\textbf{0.05985} (0.00411)&0.06077 (0.00293)&0.11238 (0.00552)\\
Car&0.18345 (0.00453)&\textbf{0.17601} (0.00163)&0.18431 (0.00303)&0.23542 (0.00072)&0.50652 (0.00330)&0.17009 (0.00174)&0.16606 (0.00402)&\textbf{0.10175} (0.00323)&0.24027 (0.00020)&0.41532 (0.00032)\\
Tableware&0.89475 (0.00284)&\textbf{0.44641} (0.00864)&0.86789 (0.00376)&0.86469 (0.00213)&0.64450 (0.00150)&\textbf{0.21437} (0.00086)&0.38609 (0.00240)&0.22125 (0.00089)&0.41498 (0.00446)&0.67902 (0.00256)\\
Ladder&0.52241 (0.00009)&0.54227 (0.00024)&0.52273 (0.00013)&0.52240 (0.00060)&\textbf{0.27069} (0.00046)&0.21872 (0.00060)&0.37963 (0.00067)&0.21957 (0.00044)&0.21828 (0.00047)&\textbf{0.13241} (0.00110)\\
Bull&0.13289 (0.00373)&0.80594 (0.00121)&\textbf{0.13217} (0.00162)&0.74641 (0.00350)&0.21890 (0.00068)&0.07061 (0.00363)&0.80143 (0.00205)&\textbf{0.06779} (0.00362)&0.79966 (0.00378)&0.10765 (0.00041)\\

\hline
\end{tabularx}
\caption{Resulting Hausdorff Distances of Different Methods for resolutions 32 and 64}
\label{resol32_64}
\end{table*}

\begin{table*}[h]
\centering
\begin{tabularx}{\textwidth}{|>{\raggedright\arraybackslash}p{2cm}|X|X|X|X||X|X|X||X|X|X|}
\hline
Name (watertight) & Num Faces & \tabularxmulticolumncentered{3}{X||}{\vspace{0pt} \large Chamfer Distance (std)} & \tabularxmulticolumncentered{3}{X||}{\vspace{0pt} \large Hausdorff Distance (std)} & \tabularxmulticolumncentered{3}{X|}{\vspace{0pt} \large Time(s)} \\ \cline{3-11} 
 &  & Diff  & 'Scan'  & DOGN  & Diff & 'Scan' & DOGN & Diff & 'Scan' & DOGN \\
\hline
Rocker-arm($\checkmark$) & 20088 & \textbf{0.02212} (0.00001) & 0.06035 (0.00007) & 0.04405 (0.00012) & \textbf{0.02875} (0.00090) & 0.10700 (0.00228) & 0.05536 (0.00158) & 24.91 & 48.49 & 14.67 \\
Beast & 64618 & \textbf{0.02020} (0.00003) & 0.06433 (0.00011) & 0.04267 (0.00005) & \textbf{0.04024} (0.00282) & 0.11064 (0.00161) & 0.08628 (0.00031) & 89.32 & 58.26 & 15.20 \\
Max Planck & 99991 & \textbf{0.02451} (0.00010) & 0.36514 (0.00189) & 0.03628 (0.00008) & 0.17925 (0.00243) & 1.07719 (0.00331) & \textbf{0.05734} (0.00065) & 139.89 & 75.70 & 18.59 \\
Lucy($\checkmark$) & 99970 & \textbf{0.01961} (0.00005) & 0.04413 (0.00020) & 0.04246 (0.00008) & \textbf{0.03140} (0.00191) & 0.11078 (0.00200) & 0.07159 (0.00016) & 139.63 & 52.06 & 13.55 \\
Cheburashka($\checkmark$) & 13334 & \textbf{0.02283} (0.00002) & 0.06890 (0.00015) & 0.04588 (0.00010) & \textbf{0.03618} (0.00377) & 0.12105 (0.00101) & 0.10863 (0.00202) & 15.71 & 60.38 & 16.87 \\
Happy & 98601 & \textbf{0.02165} (0.00007) & 0.06306 (0.00022) & 0.04383 (0.00008) & \textbf{0.03353} (0.00252) & 0.15536 (0.00016) & 0.05918 (0.00079) & 137.77 & 55.52 & 15.53 \\
Teapot & 6320 & \textbf{0.02224} (0.00002) & 0.21243 (0.00083) & 0.04506 (0.00018) & 0.10466 (0.00050) & 1.00711 (0.00192) & \textbf{0.10269} (0.00028) & 7.47 & 68.04 & 14.69 \\
Bimba($\checkmark$) & 224906 & \textbf{0.02426} (0.00006) & 0.09357 (0.00016) & 0.04720 (0.00009) & \textbf{0.03871} (0.00186) & 0.12011 (0.00015) & 0.06437 (0.00091) & 374.64 & 75.76 & 17.81 \\
Igea($\checkmark$) & 268686 & \textbf{0.02575} (0.00006) & 0.13466 (0.00015) & 0.05147 (0.00011) & \textbf{0.03688} (0.00157) & 0.11490 (0.00136) & 0.06003 (0.00266) & 451.48 & 87.85 & 18.27 \\
Hourse($\checkmark$) & 96966 & \textbf{0.02130} (0.00000) & 0.08847 (0.00019) & 0.04442 (0.00012) & \textbf{0.03175} (0.00265) & 0.60367 (0.00467) & 0.05657 (0.00138) & 135.42 & 66.81 & 14.92 \\
Homer($\checkmark$) & 12000 & \textbf{0.02014} (0.00001) & 0.05297 (0.00021) & 0.04231 (0.00009) & \textbf{0.02928} (0.00239) & 0.10570 (0.00048) & 0.09825 (0.00138) & 14.13 & 53.53 & 13.99 \\
Spot & 5856 & \textbf{0.02442} (0.00010) & 0.09000 (0.00012) & 0.04708 (0.00004) & \textbf{0.03489} (0.00044) & 0.11879 (0.00149) & 0.05470 (0.00110) & 6.93 & 66.23 & 14.88 \\
Armadillo($\checkmark$) & 99976 & \textbf{0.02365} (0.00009) & 0.07687 (0.00006) & 0.04697 (0.00010) & \textbf{0.03633} (0.00140) & 0.12065 (0.00033) & 0.05840 (0.00132) & 139.45 & 61.74 & 15.53 \\
Suzanne & 968 & \textbf{0.02423} (0.00001) & 0.09001 (0.00010) & 0.04917 (0.00018) & \textbf{0.08368} (0.00175) & 0.58039 (0.00234) & 0.11331 (0.00174) & 1.19 & 64.79 & 13.75 \\
Stanford Bunny & 69451 & \textbf{0.02668} (0.00004) & 0.18646 (0.00057) & 0.03927 (0.00010) & 0.09665 (0.00154) & 0.79551 (0.00374) & \textbf{0.06049} (0.00240) & 96.41 & 71.52 & 17.91 \\
Nefertiti($\checkmark$) & 99938 & \textbf{0.02221} (0.00003) & 0.07914 (0.00014) & 0.04485 (0.00004) & \textbf{0.03048} (0.00077) & 0.10623 (0.00101) & 0.06128 (0.00267) & 139.66 & 81.66 & 15.88 \\
Ogre & 124008 & \textbf{0.02241} (0.00004) & 0.06616 (0.00023) & 0.04644 (0.00016) & \textbf{0.09947} (0.00153) & 0.12944 (0.00218) & 0.13369 (0.00087) & 175.89 & 59.81 & 14.76 \\
Cow($\checkmark$) & 5804 & \textbf{0.02030} (0.00002) & 0.21046 (0.00219) & 0.04294 (0.00011) & \textbf{0.03217} (0.00083) & 0.95843 (0.00681) & 0.05663 (0.00025) & 6.88 & 52.27 & 13.42 \\
Fandisk($\checkmark$) & 12946 & \textbf{0.02753} (0.00005) & 0.08065 (0.00017) & 0.04490 (0.00013) & \textbf{0.03944} (0.00156) & 0.47152 (0.00420) & 0.06074 (0.00087) & 15.23 & 50.06 & 13.78 \\
Car & 157384 & \textbf{0.03895} (0.00022) & 0.08014 (0.00016) & 0.06685 (0.00001) & 0.16614 (0.00562) & \textbf{0.15815} (0.00457) & 0.19055 (0.00186) & 231.67 & 52.94 & 18.01 \\
Tableware & 4788 & \textbf{0.06436} (0.00009) & 0.08177 (0.00029) & 0.21082 (0.00053) & \textbf{0.18588} (0.00271)& 0.20589 (0.01163)&0.69894 (0.00030) & 5.70 & 41.63 & 13.12 \\
Ladder & 828 & \textbf{0.02767} (0.00005) & 0.08104 (0.00014) & 0.04041 (0.00010) & \textbf{0.04449} (0.00106) & 0.14899 (0.00062) & 0.06803 (0.00132) & 2.40 & 30.80 & 13.08 \\
Bull & 2418 & \textbf{0.02309} (0.00007) & 0.20242 (0.00165) & 0.04534 (0.00008) & \textbf{0.03539} (0.00165) & 0.81664 (0.00358) & 0.05535 (0.00029) & 2.91 & 56.92 & 15.08 \\
\hline
\end{tabularx}
\caption{Resulting Chamfer Distances, Hausdorff Distances, and Computation Times of Different Methods for resolution 128}
\label{table_resol128}
\end{table*}

\begin{table*}[h]
\centering
\begin{tabularx}{\textwidth}{|>{\raggedright\arraybackslash}p{2cm}|X|X|X|X||X|X|X||X|X|X|}
\hline
Name (watertight) & Num Faces & \tabularxmulticolumncentered{3}{X||}{\vspace{0pt} \large Chamfer Distance (std)} & \tabularxmulticolumncentered{3}{X||}{\vspace{0pt} \large Hausdorff Distance (std)} & \tabularxmulticolumncentered{3}{X|}{\vspace{0pt} \large Time(s)} \\ \cline{3-11} 
 &  & Diff  & 'Scan'  & DOGN  & Diff & 'Scan' & DOGN & Diff & 'Scan' & DOGN \\
\hline
Rocker-arm($\checkmark$) & 20088 & \textbf{0.01702} (0.00008) & 0.05966 (0.00015) & 0.02648 (0.00006) & \textbf{0.02691} (0.00079) & 0.10362 (0.00084) & 0.03337 (0.00053) & 198.46 & 306.67 & 103.14 \\
Beast & 64618 & \textbf{0.01502} (0.00007) & 0.06272 (0.00013) & 0.02526 (0.00002) & \textbf{0.02309} (0.00102) & 0.10318 (0.00027) & 0.08098 (0.00022) & 744.10 & 368.34 & 107.00 \\
Max Planck & 99991 & \textbf{0.02033} (0.00002) & 0.37075 (0.00201) & 0.02555 (0.00002) & 0.18064 (0.00128) & 1.08849 (0.00818) & \textbf{0.03709} (0.00180) & 1158.30 & 484.46 & 135.59 \\
Lucy($\checkmark$) & 99970 & \textbf{0.01501} (0.00003) & 0.04233 (0.00019) & 0.02463 (0.00005) & \textbf{0.02503} (0.00066) & 0.11022 (0.00372) & 0.04462 (0.00083) & 1155.86 & 345.91 & 111.01 \\
Cheburashka($\checkmark$) & 13334 & \textbf{0.01806} (0.00003) & 0.06823 (0.00002) & 0.02769 (0.00012) & \textbf{0.02977} (0.00083) & 0.16839 (0.00756) & 0.08520 (0.00111) & 130.68 & 392.88 & 121.58 \\
Happy & 98601 & \textbf{0.01726} (0.00003) & 0.06299 (0.00017) & 0.02656 (0.00004) & \textbf{0.02687} (0.00076) & 0.15838 (0.00108) & 0.03588 (0.00088) & 1140.47 & 319.96 & 114.05 \\
Teapot & 6320 & \textbf{0.01757} (0.00007) & 0.25775 (0.00125) & 0.02353 (0.00005) & 0.10390 (0.00108) & 1.01302 (0.00292) & \textbf{0.03257} (0.00040) & 61.94 & 462.17 & 114.65 \\
Bimba($\checkmark$) & 224906 & \textbf{0.02056} (0.00006) & 0.09320 (0.00020) & 0.02989 (0.00010) & \textbf{0.03400} (0.00125) & 0.11556 (0.00130) & 0.03926 (0.00236) & 3050.98 & 455.75 & 135.22 \\
Igea($\checkmark$) & 268686 & \textbf{0.02164} (0.00006) & 0.13443 (0.00021) & 0.03212 (0.00002) & 0.04057 (0.00378) & 0.10788 (0.00041) & \textbf{0.03991} (0.00023) & 3649.88 & 534.83 & 135.75 \\
Hourse($\checkmark$) & 96966 & \textbf{0.01587} (0.00002) & 0.08751 (0.00038) & 0.02600 (0.00005) & \textbf{0.02425} (0.00024) & 0.60148 (0.00601) & 0.03771 (0.00162) & 1120.32 & 418.90 & 115.71 \\
Homer($\checkmark$) & 12000 & \textbf{0.01507} (0.00001) & 0.05253 (0.00008) & 0.02510 (0.00003) & \textbf{0.02412} (0.00045) & 0.09813 (0.00144) & 0.07579 (0.00068) & 117.49 & 341.66 & 107.74 \\
Spot & 5856 & \textbf{0.01996} (0.00005) & 0.08974 (0.00039) & 0.02957 (0.00008) & \textbf{0.03278} (0.00201) & 0.11833 (0.00163) & 0.03788 (0.00242) & 57.42 & 441.26 & 120.16 \\
Armadillo($\checkmark$) & 99976 & \textbf{0.01876} (0.00003) & 0.07367 (0.00021) & 0.02858 (0.00005) & \textbf{0.03146} (0.00101) & 0.11894 (0.00291) & 0.03571 (0.00052) & 1155.40 & 356.79 & 121.72 \\
Suzanne & 968 & \textbf{0.01947} (0.00003) & 0.09038 (0.00011) & 0.03012 (0.00013) & \textbf{0.08047} (0.00191) & 0.58337 (0.00194) & 0.09545 (0.00056) & 9.79 & 430.40 & 108.23 \\
Stanford Bunny & 69451 & \textbf{0.02215} (0.00004) & 0.20425 (0.00038) & 0.02847 (0.00014) & 0.10349 (0.00072) & 0.84211 (0.00584) & \textbf{0.04049} (0.00102) & 802.02 & 479.98 & 130.56 \\
Nefertiti($\checkmark$) & 99938 & \textbf{0.01779} (0.00001) & 0.08017 (0.00040) & 0.02747 (0.00006) & \textbf{0.03064} (0.00078) & 0.10384 (0.00123) & 0.03866 (0.00489) & 1156.84 & 560.41 & 118.79 \\
Ogre & 124008 & \textbf{0.01711} (0.00006) & 0.06440 (0.00019) & 0.02906 (0.00010) & \textbf{0.07934} (0.01013) & 0.13050 (0.00250) & 0.12526 (0.00099) & 1441.33 & 375.40 & 112.09 \\
Cow($\checkmark$) & 5804 & \textbf{0.01534} (0.00004) & 0.21486 (0.00047) & 0.02528 (0.00006) & \textbf{0.02932} (0.00096) & 0.95404 (0.00273) & 0.04360 (0.00044) & 57.02 & 354.76 & 105.84 \\
Fandisk($\checkmark$) & 12946 & \textbf{0.02054} (0.00007) & 0.08235 (0.00028) & 0.03002 (0.00006) & \textbf{0.03789} (0.00251) & 0.48765 (0.00281) & 0.04194 (0.00159) & 127.07 & 321.94 & 107.73 \\
Car & 157384 & \textbf{0.03552} (0.00008) & 0.07919 (0.00037) & 0.04584 (0.00010) & 0.16396 (0.00319) & \textbf{0.16026} (0.00826) & 0.18403 (0.00240) & 1849.66 & 285.01 & 129.18 \\
Tableware & 4788 & \textbf{0.01938} (0.00005) & 0.05631 (0.00012) & 0.20433 (0.00199) & \textbf{0.04357} (0.00273)& 0.17771 (0.00911)& 0.70841 (0.00024) & 47.18 & 247.94 & 102.09 \\
Ladder & 828 & \textbf{0.01530} (0.00004) & 0.06477 (0.00031) & 0.02357 (0.00009) & \textbf{0.02224} (0.00056) & 0.12011 (0.00055) & 0.03213 (0.00047) & 16.29 & 156.47 & 101.86 \\
Bull & 2418 & \textbf{0.01802} (0.00002) & 0.21368 (0.00172) & 0.02774 (0.00003) & \textbf{0.02930} (0.00056) & 0.81471 (0.00494) & 0.03632 (0.00185) & 24.04 & 373.57 & 112.22 \\
\hline
\end{tabularx}
\caption{Resulting Chamfer Distances, Hausdorff Distances, and Computation Times of Different Methods for resolution 256}
\label{table_resol256}
\end{table*}

\section{Rationale}
\label{sec:rationale}
Having the supplementary compiled together with the main paper means that:
\begin{itemize}
\item The supplementary can back-reference sections of the main paper, for example, we can refer to \cref{sec:intro};
\item The main paper can forward reference sub-sections within the supplementary explicitly (e.g. referring to a particular experiment); 
\item When submitted to arXiv, the supplementary will already included at the end of the paper.
\end{itemize}
To split the supplementary pages from the main paper, you can use \href{https://support.apple.com/en-ca/guide/preview/prvw11793/mac#:~:text=Delete%20a%20page%20from%20a,or%20choose%20Edit%20%3E%20Delete).}{Preview (on macOS)}, \href{https://www.adobe.com/acrobat/how-to/delete-pages-from-pdf.html#:~:text=Choose%20%E2%80%9CTools%E2%80%9D%20%3E%20%E2%80%9COrganize,or%20pages%20from%20the%20file.}{Adobe Acrobat} (on all OSs), as well as \href{https://superuser.com/questions/517986/is-it-possible-to-delete-some-pages-of-a-pdf-document}{command line tools}.
